# Supplementary material for: Exploiting Stability-Plasticity Asymmetry in Pretrained Detectors for Incremental Object Detection
Source: arXiv:2504.10214 source file (2026-09-01)
Supplement: Supplementary file 1 [file table_appendix.tex]

\begin{table*}
\caption{mAP@50 results of VOC and TT100K. The best result in each column is \textbf{bolded}, and the second-best result is \underline{underlined}. Methods with $^\dagger$ means results of VOC from our re-implementation.}
\label{tab:tt100k_voc_appendix}
\centering
\centering
\footnotesize
%\resizebox{\textwidth}{!}{
\begin{tabular}{l|lll|lll||lll|lll} 
\hline
\multicolumn{1}{l|}{\textbf{Dataset}} & \multicolumn{6}{c||}{\textbf{VOC}} & \multicolumn{6}{c}{\textbf{TT100K}} \\ 
\hline
\textbf{Setting} & \multicolumn{3}{c|}{\textbf{10-10 (2 Tasks)}} & \multicolumn{3}{c||}{\textbf{10-2 (6 Tasks)}} & \multicolumn{3}{c|}{\textbf{10-10 (2 Tasks)}} & \multicolumn{3}{c}{\textbf{10-2 (6 Tasks)}} \\ 
\hline
\textbf{Method} & \textbf{1-10} & \textbf{11-20} & \cellcolor{gray!30} \textbf{1-20}  & \textbf{1-10} & \textbf{11-20} & \cellcolor{gray!30} \textbf{1-20} & \textbf{1-10} & \textbf{11-20} & \cellcolor{gray!30} \textbf{1-20} & \textbf{1-10} & \textbf{11-20} & \cellcolor{gray!30} \textbf{1-20} \\ 
\hline
Faster ILOD & 70.3 & 53.0 & \cellcolor{gray!30} 61.7 & 64.2 & 48.6 & \cellcolor{gray!30} 56.4 & 49.1 & 21.2 & \cellcolor{gray!30} 35.2 & 47.5 & 13.5 & \cellcolor{gray!30} 30.5 \\
MMA & 69.8 & 63.9 & \cellcolor{gray!30} 66.8 & 65.7 & 52.5 & \cellcolor{gray!30} 59.1 & 48.1 & 28.0 & \cellcolor{gray!30} 38.1 & 45.3 & 17.6 & \cellcolor{gray!30} 31.4  \\
ABR & 71.2 & 72.8 & \cellcolor{gray!30} 72.0 & \underline{67.0} & \underline{58.1} & \cellcolor{gray!30} \underline{62.6} & \underline{55.0} & \underline{39.3} & \cellcolor{gray!30} \underline{47.2} & \underline{48.3} & \underline{22.0} & \cellcolor{gray!30} \underline{35.2} \\
CL-DETR$^\dagger$ & 45.2 & 56.0 & \cellcolor{gray!30} 50.6 & 32.0 & 17.4 & \cellcolor{gray!30} 24.7 & 52.1 & 37.5 & \cellcolor{gray!30} 44.8 & 39.4 & 8.2 & \cellcolor{gray!30} 23.8 \\
MD-DETR$^\dagger$ & \underline{81.8} & \underline{87.3} & \cellcolor{gray!30} \underline{84.6} & 30.7 & 37.1 & \cellcolor{gray!30} 33.9 & 0.1 & 37.1 & \cellcolor{gray!30} 18.6 & 0 & 7.5 & \cellcolor{gray!30} 3.7 \\
\hline
\hline
Ours & \textbf{94.4} & \textbf{90.7} & \cellcolor{gray!30} \textbf{92.5} & \textbf{93.6} & \textbf{89.9} & \cellcolor{gray!30} \textbf{91.8} & \textbf{77.8} & \textbf{51.5} & \cellcolor{gray!30} \textbf{64.6} & \textbf{76.2} & \textbf{43.6} & \cellcolor{gray!30} \textbf{59.9} \\
\hline
\end{tabular}
% }
\end{table*}
